# Supplementary material for: Sharing without Showing: Secure Cloud Analytics with Trusted Execution Environments
Source: arXiv:2410.10574 source file (2024-10-14)
Supplement: Supplementary file 1 [file appendix.tex]

\section{Taxi distribution evaluation}
\label{sec:taxi_simulation}
In this section, we show an idea of how the taxi distribution use case can be visualized. 

In Figure \ref{fig:taxi_simulation} we represent 3 different views in this simulation. In Figure \ref{fig:taxi_distribution}, we show the distribution of taxis at a given moment. This data could be valuable for citizens to know where it is easier or harder to get a taxi, as well as for the taxi companies, to know where it is best to send their taxis.

In Figure \ref{fig:company_view} we show the view from one of the taxi companies.

In Figure \ref{fig:global_view} we show a subset of all taxis from the simulation. This view is not possible to see for anyone since one needs to be in possession of all keys from the different taxi companies, something that no party has access to.

Knowing where the traffic flows and where there currently is traffic congestion in real-time is valuable knowledge for every vehicle currently in traffic.
To get this information, one could monitor everyone's position and detect when traffic is moving slower. However, such approaches would violate the privacy of the user, since the position data has to be shared broadly. At the same time, it is not necessary to know the position of all vehicles in traffic to detect a traffic jam. By using only the position of taxi cars, one can get an idea of where the traffic flows while not monitoring every individual person. This data can also be used by the taxi companies themselves to both monitor where their own vehicles are, and to get a view of which zones currently have more or fewer taxi cars. The public could use the information to know both about traffic congestion and taxi availability.

\begin{figure}
    \centering
  \subfloat[Public view of taxi distribution in different zones in a city.\label{fig:taxi_distribution}]{%
\begin{minipage}{\columnwidth}
\centering    \includegraphics[trim={19mm 20mm 25mm 18mm},clip, width=0.8\columnwidth]{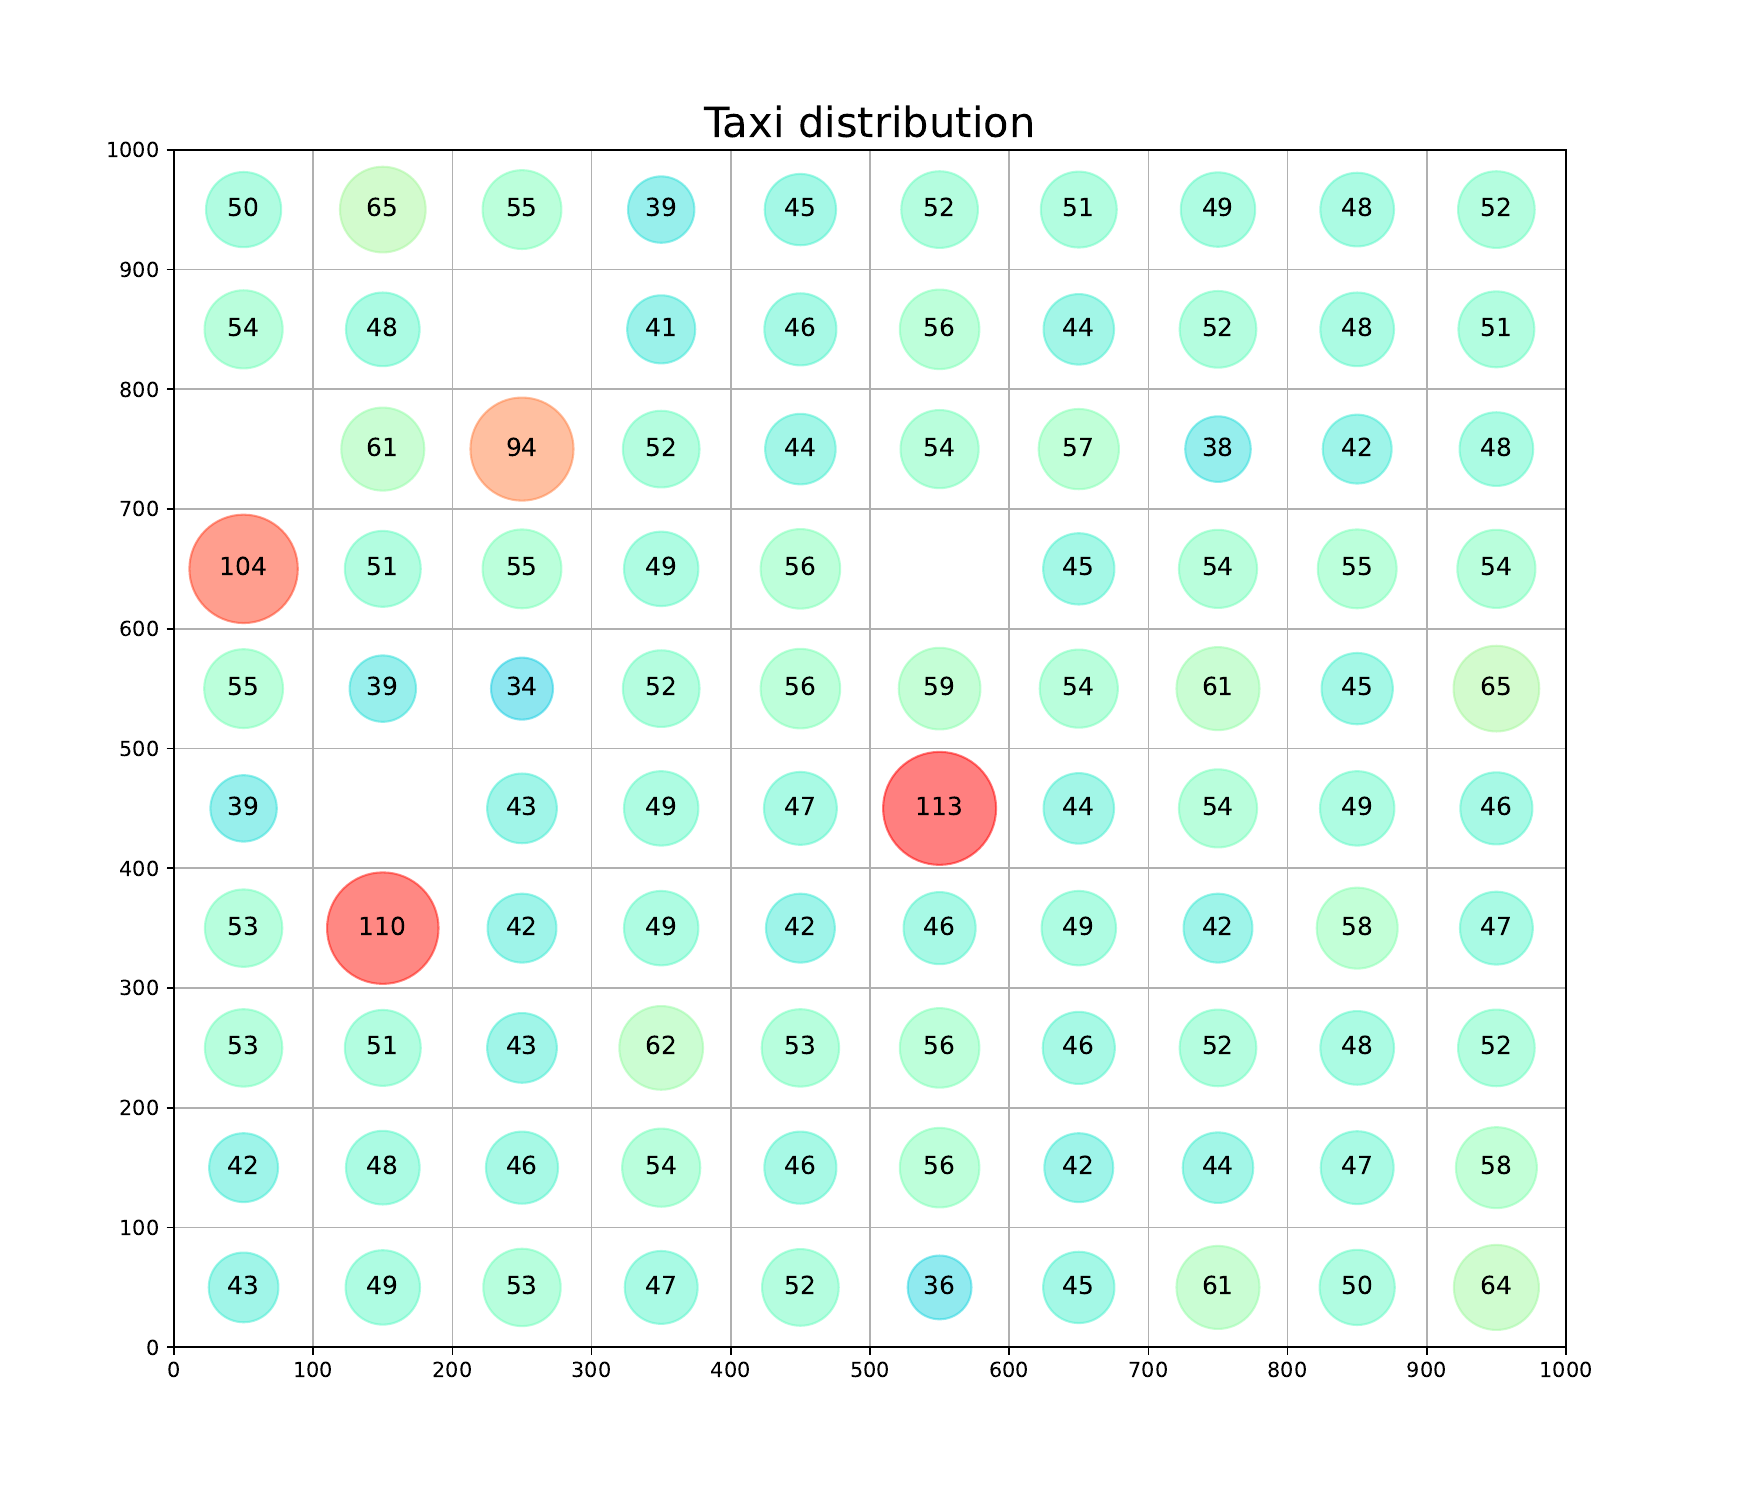}
\end{minipage}}
    %% \hfill
  \hspace{-11mm}
  \subfloat[Real-time view of one company's taxi cars.\label{fig:company_view}]{%
\begin{minipage}{\columnwidth}
% \centering        \includegraphics[scale=0.75]{authorization}
  \centering        \includegraphics[trim={21mm 21mm 31mm 19mm},clip,width=0.8\columnwidth]{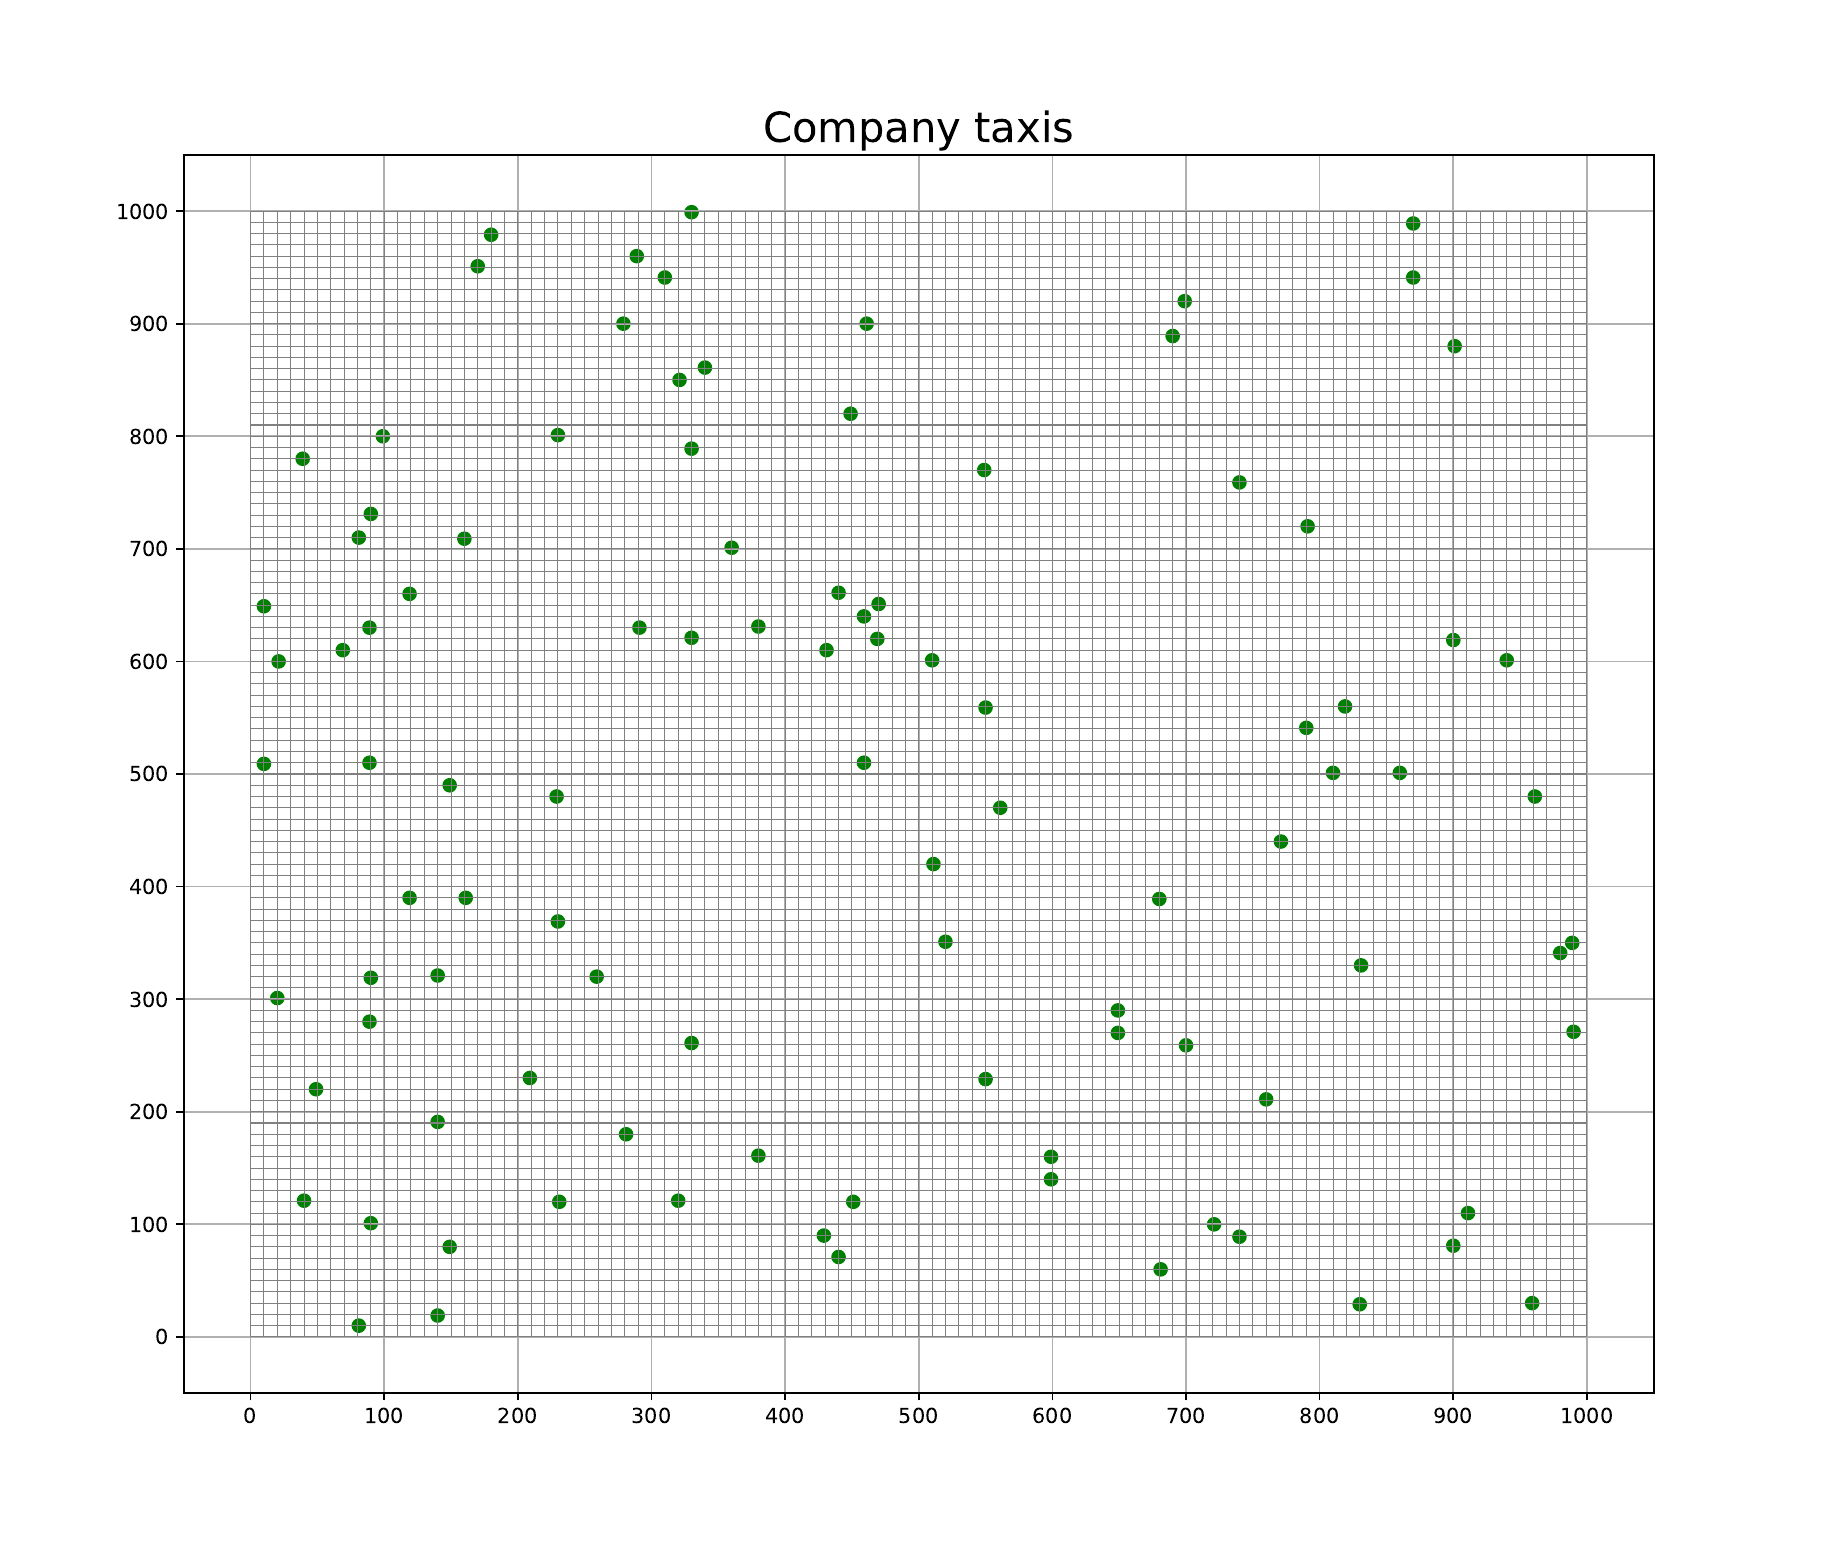}
\end{minipage}}
   %% \hfill
  \hspace{1mm}
   \subfloat[Global view (not visible by anyone) of taxis from 5 different companies.\label{fig:global_view}]{%
\begin{minipage}{\columnwidth}
\centering        \includegraphics[trim={19mm 20mm 28mm 18mm},clip,width=0.8\columnwidth]{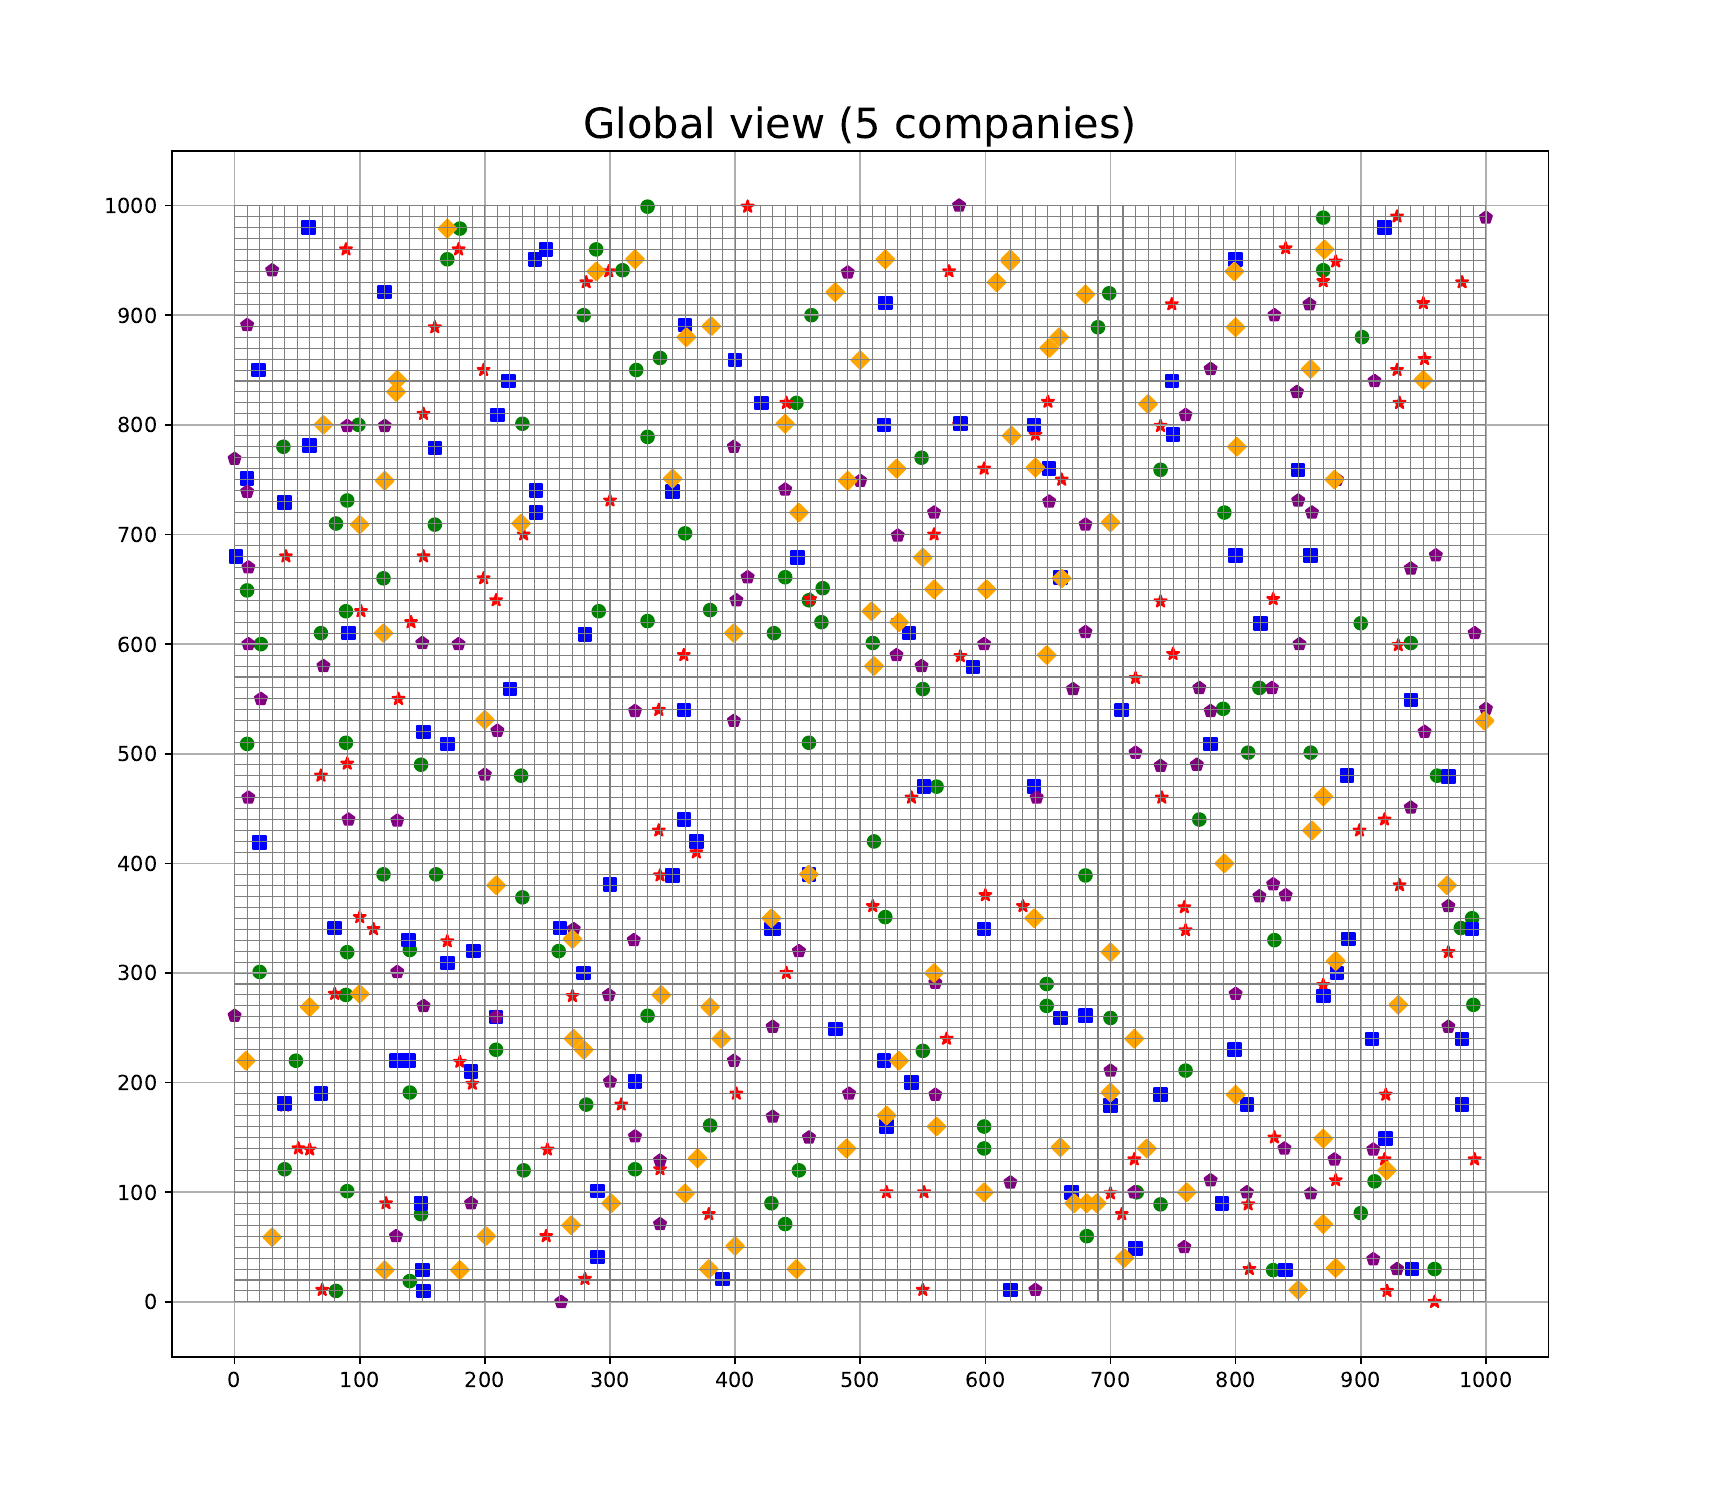}
\end{minipage}}
  \caption{Different views of the real-time position of taxi cars. The public view (Fig.~\ref{fig:taxi_distribution}) shows only the number of taxis in each zone. Each company (Fig.~\ref{fig:company_view}) that can only access the position of their own cars. While all data can be aggregated, a global view (Fig.~\ref{fig:global_view}) is not accessible unless all data is public.}
  \label{fig:taxi_simulation} 
  %% \hfill
\end{figure}
